# Supplementary material for: Combining Electromagnetic and Gravitational-Wave Constraints on Neutron-Star Masses and Radii
Source: arXiv:2008.12817 source file (2020-11-17)
Supplement: Supplementary file 1 [file supp.pdf]

# Combining Electromagnetic and Gravitational-Wave Constraints on Neutron-Star Masses and Radii: Supplemental Material

Mohammad Al-Mamun[1], Andrew W. Steiner[1], Joonas Nättilä[2,3], Jacob Lange[4], Richard O'Shaugnessy[4], Ingo Tews[5], Stefano Gandolfi[5], Craig Heinke[6], and Sophia Han[7,8]

[1] *Department of Physics and Astronomy, University of Tennessee, Knoxville, TN 37996, USA*
[2] *Physics Department and Columbia Astrophysics Laboratory, Columbia University, 538 West 120th Street, New York, NY 10027, USA*
[3] *Center for Computational Astrophysics, Flatiron Institute, 162 Fifth Avenue, New York, NY 10010, USA*
[4] *Rochester Institute of Technology, 85 Lomb Memorial Drive, Rochester, NY 14623, USA*
[5] *Theoretical Division, Los Alamos National Laboratory, Los Alamos, NM 87545, USA*
[6] *U. Alberta, 116 St. and 85 Ave., Edmonton, AB, Canada*
[7] *Department of Physics, University of California, Berkeley, CA 94720, USA and*
[8] *Department of Physics and Astronomy, Ohio University, Athens, OH 45701, USA*

## METHOD

### Probability distributions from NS observations

As in Refs. [1, 2], we include mass and radius constraints from seven quiescent low mass X-ray binaries (QLMXBs) in the globular clusters 47 Tuc (the QLMXB X7), $\omega$ Cen, NGC 6397, NGC 6304, M 13, M 28, and M 30. We include distance uncertainties, and the possibility for either H or He atmospheres as in Ref. [1], but we assume that the temperature is uniform and do not consider the possible effects of hotspots (we do not assume a uniform temperature distribution for the NICER source J0030+0451 below).

We include mass-radius constraints from PRE X-ray bursters SAX J1810.8−429 and 4U 1724−307 performed using the cooling-tail method [3]. We also include mass and radius constraints from Ref. [4] on the PRE X-ray burster 4U 1702−429, obtained using the direct atmosphere model fit method. We focus only on their model "D" results: this corresponds to a parameter optimization with the most relaxed initial prior assumptions where the hydrogen fraction is treated as a free parameter.

Refs. [5, 6] obtained mass and radius constraints using an analysis of NICER X-ray timing data on PSR J0030+0451. We used the results from Ref. [5], but expect that results using the constraints from Ref. [6] would be similar.

The X-ray observations may not include all of the systematics. Our analysis combines mass and radius constraints which were obtained from different methods, and this combination mitigates some of these systematics. A method to quantify additional unknown systematics is to fold an additional intrinsic uncertainty in both the mass and the radius for each measurement. In our case, this would require an additional 22 parameters (or 24 parameters with the NICER data). We find that this larger parameter space increases the computational cost significantly. To moderate this cost, we define a single Intrinsic Scattering (IS) parameter, $\sigma$, for each neutron star. We fix the width of the Gaussian in the mass direction to be $\sigma_M \equiv (1.4\ \mathrm{M}_\odot)\sigma$ and the width in the radius direction to be $\sigma_R \equiv (5\ \mathrm{km})\sigma$. Thus, there is only one coupled intrinsic scattering parameter for each neutron star for which we have EM data. Using this, the two-dimensional probability distribution for the mass and radius, $\mathcal{D}(\mathcal{R},\mathcal{M})$ is modified to

$$\mathcal{D}_{\mathrm{IS}}(R,M,\sigma) = \frac{1}{\mathcal{N}}\int_{R_0}^{R_1}\int_{M_0}^{M_1} dR'\ dM'\mathcal{D}(R',M') \times \exp\left[-\frac{1}{2}\left(\frac{R-R'}{\sigma_R}\right)^2 - \frac{1}{2}\left(\frac{M-M'}{\sigma_M}\right)^2\right], \quad (1)$$

where $\mathcal{N} = \int_V D_{\mathrm{IS}}\ dV$ is a normalization factor preserving the probability density over the total volume $V$. We note that in theory $\mathcal{N}$ is just a normalization related to an integral over a multivariate Gaussian, but in practice the finite boundary effects complicate it therefore it is easiest to evaluate the integral numerically. There are several alternatives for the procedure which we chose. One could express the uncertainty in terms of the compactness $M/R$ or the GR-corrected radius $R_\infty = R\left(1-2GM/Rc^2\right)^{-1/2}$ instead of $M$ and $R$. Also, one could choose a different smoothing kernel than a Gaussian function. Different choices of the kernel or the variables on which the Gaussian is written would particularly impact the tails of the posterior distributions. An examination of alternatives, however, will be left to future work.

For the data from GW170817 [7], we interpolate a marginal likelihood for binary parameters $\mathcal{M}_{\mathrm{det}}, \delta m, \tilde{\Lambda}, \chi_{1,z}, \chi_{2,z}$, integrating over nuisance extrinsic parameters like source orientation relative to the line of sight. Provided by RIFT [8], this marginal likelihood is a function of the dimensionless NS spins $\chi_{i,z}$ relative to the orbital angular momentum direction $\hat{L} = \hat{z}$, the binary chirp mass in the detector frame

$$\mathcal{M}_{\mathrm{det}} = \frac{(M_1 M_2)^{3/5}}{(M_1+M_2)^{1/5}}(1+z) \quad (2)$$

where $z$ is the redshift of the merger, the mass difference $\delta m \equiv M_1 - M_2$, and the combined tidal deformability

$$\tilde{\Lambda} = \frac{16}{13} \frac{(M_1 + 12M_2)\, M_1^4 \Lambda_1 + (M_2 + 12M_1)\, M_2^4 \Lambda_2}{(M_1 + M_2)^5} \,. \tag{3}$$

Empirically, the marginal likelihood for GW170817 does not appreciably depend on the antisymmetric combination $\Delta\tilde{\Lambda}$. We then further marginalize this five-dimensional over the two dimensionless spins to produce a three-dimensional marginal likelihood which depends only on $\mathcal{M}_{\rm det}, \delta m, \tilde{\Lambda}$.

As discussed in Refs. [9, 10], we require an additional nuisance parameter for each neutron star, which we choose to be the mass: $M_1$ and $M_2$, for the neutron stars involved in GW170817, and $M_3, M_4, \ldots$ for the neutron stars which have photon-based mass and radius constraints. In addition, the QLMXBs have an additional parameter $\eta_i$ which chooses between a H or He atmosphere for each particular object $i$. Presuming our EOS model has parameters $\{p\}$, the conditional probability is just the product

$$\begin{aligned} \mathcal{P}(D|M) = D_{\rm LIGO}\, &[\mathcal{M}_{\rm det}(M_1, M_2, z), \delta m(M_1, M_2), \\ &\tilde{\Lambda}(M_1, M_2, \{p\})\Big] \\ &\times \prod_{i=3}^{N+3} D_{\rm i}[R(M_i, \{p\}), M_i, \eta_i, \sigma_i] \end{aligned} \tag{4}$$

where $P_{\rm QMC}$ is described below and $N$ is 11 when the NICER data is included and 10 otherwise.

All prior probability distributions are flat between boundaries which do not impact the final results, except for (i) the parameters $a, \alpha, b,$ and $\beta$ (described below) which follow a multivariate Gaussian distribution, (ii) the intrinsic scattering parameters which are flat in $\log_{10} \sigma_i$ between $-2$ and 2, and (iii) the redshift of GW170817 which is a Gaussian distribution with peak at 0.0099 and width of 0.0009 [7]. Our full prior probability also contains several choices about our model construction which are described below.

## EOS Model

We describe nuclear matter near saturation with an approach very similar to that from Ref. [11]. For this, we need to model both pure neutron matter (PNM) and symmetric nuclear matter (SNM). Pure neutron matter (i.e., vanishing proton fraction) can be well-described with a parameterization proposed in Ref. [12];

$$E_{\rm PNM}(n_{\rm B}) = a \left(\frac{n_{\rm B}}{n_0}\right)^{\alpha} + b \left(\frac{n_{\rm B}}{n_0}\right)^{\beta} \,. \tag{5}$$

In order to recast the parameters in terms of the symmetry energy $S$ and its derivative $L$, we use the relations

$$\begin{aligned} S &= a + b + 16 \text{ MeV} \\ L &= 3(a\alpha + b\beta) \,. \end{aligned} \tag{6}$$

We selected parameter sets for $a, \alpha, b,$ and $\beta$ based on the neutron-matter calculations of Ref. [13], where local chiral EFT interactions of Refs. [14, 15] were combined with the auxiliary field diffusion Monte Carlo method [16] to obtain the energy per particle of neutron matter with theoretical uncertainty estimates. The parameters $a, b, \alpha$ and $\beta$ are selected from uniform priors in the intervals $[0, 20]$, $[0, 20]$, $[0, 1]$ and $[1, 10]$, respectively. For each parameter set, we check if the resulting curve for $E_{\rm PNM}(n_{\rm B})$ falls within the uncertainty band of Ref. [13] in the density range from $(0.5 - 1.0)\; n_0$. In addition, we check if the resulting pressure at saturation density falls within the predicted range. For all $\mathcal{O}(1000)$ parameter sets that pass these tests, we fit the probability distribution to a four-dimensional Gaussian, and then select those four parameters according to that Gaussian distribution. For symmetric nuclear matter (i.e., equal neutron and proton fractions) we select a random Skyrme model from a list of 1000 models provided by the authors of Ref. [17] (see also Ref. [18]). Our final nuclear-matter EOS is then given by

$$\begin{aligned} E(n_{\rm B}, x) = E_{\rm Skyrme}(n_{\rm B}, x = 0.5) + [(1 - 2x)^2 E_{\rm PNM}(n_{\rm B}) \\ - E_{\rm Skyrme}(n_{\rm B}, x = 0.5)] \,. \end{aligned} \tag{7}$$

To construct neutron-star matter, we determine the proton fraction in beta-equilibrium by ensuring that $\mu_n = \mu_p + \mu_e$.

For higher densities, we use two different EOS parameterizations. The first is an EOS based on three polytropic segments, each given by $P = K\epsilon^{\Gamma}$, where the adiabatic index $\Gamma \equiv 1 + 1/n$ and $n$ is the polytropic index. This model is similar to Model A of Refs. [1, 19] and also similar to that from Ref. [20] as used by the LIGO and VIRGO collaborations in Ref. [7]. The QMC results are used up to the energy density which corresponds to twice the nuclear saturation density. Beyond that energy density, the first polytrope, with index $n_1$, is used. The second polytrope, with index $n_2$, begins at energy density $\varepsilon_1$, and ends at energy density $\varepsilon_2$. The third polytrope, with index $n_3$, is used for all higher energy densities. We use uniform prior distributions for these five EOS parameters. The coefficients $K$ are fixed to ensure the EOS is continuous. This model is labeled "3P" below.

There may be a phase transition in high-density matter, but strong phase transitions imply extreme values of $\Gamma$ and $K$ in polytropic models and, thus, are disfavored by our choice of uniform prior distributions. Therefore, we choose an alternative EOS parametrization which more naturally includes phase transitions. In this parameterization, the EOS is constructed by a set of line segments

| Label | EOS parameterizations and data selection |
|---|---|
| (a) | 3P with GW only |
| (b) | 4L with GW only |
| (c) | 3P with {GW, QLMXB, PRE} |
| (d) | 4L with {GW, QLMXB, PRE} |
| (e) | 3P with {GW, QLMXB, PRE, NICER} |
| (f) | 4L with {GW, QLMXB, PRE, NICER} |
| (g) | 3P with {GW, QLMXB, PRE, NICER} w/int. scat. |
| (h) | 4L with {GW, QLMXB, PRE, NICER} w/int. scat. |

TABLE I. Legend explaining EOS parameterizations and data sets used in the figures. The three-polytrope model is labeled "3P", and the four line-segment model is labeled "4L".

which change slope at fixed energy densities, 400, 600, and 1000 MeV/fm$^3$. The first line segment begins at the energy density which corresponds to twice the nuclear saturation density and has pressure $P_1$ at 400 MeV/fm$^3$. The next three line segments have pressures $P_2$, $P_3$, and $P_4$ at energy densities of 600, 1000, and 1400 MeV/fm$^3$, respectively. We choose uniform prior distributions for these four pressure parameters. This model is labeled "4L" below.

Finally, the dimensionless speed of sound squared, $c_s^2/c^2 = dP/d\epsilon$ is constrained to be between 0 and 1 at all densities below the central pressure of the maximum-mass neutron star.

## Neutron-star structure

We presume the neutron stars are spherical, non-rotating, objects with $T = 0$. The Tolman-Oppenheimer-Volkov (TOV) equations [21, 22] are solved to compute the neutron-star mass and radius as a function of the central pressure. We ensure the maximum mass is at least two solar masses in our baseline calculation in order to match recent observations of high-mass neutron stars [23–25]. Ref. [25] implies a larger mass, $2.14^{+0.10}_{-0.09}$ M$_\odot$, but also a larger uncertainty. We can always refine the selection of posterior samples to increase the maximum mass if necessary. We compute the moment of inertia as a function of the gravitational mass using the Hartle approximation [26]. Ref. [27] showed the existence of a strong correlation between the scaled moment of inertia ($\bar{I} \equiv I/M^3$) and the scaled tidal Love deformability ($\bar{\Lambda} \equiv \lambda/M^5$). We use the relation provided in Ref. [28] to calculate the dimensionless tidal deformabilities of the NSs;

$$\ln\ \bar{\Lambda} \simeq -30.5395 + 38.3931\ (\ln \bar{I}) - 16.307\ (\ln \bar{I})^2 + 3.36972\ (\ln \bar{I})^3 - 0.26105\ (\ln \bar{I})^4 \qquad (8)$$

See also Ref. [29] for an updated analysis on the relationship between $\bar{I}$ and $\bar{\Lambda}$.

## Computational details

We use the affine-invariant sampling method proposed by Ref. [30] which simulates the object function with an ensemble of "walkers". This sampling method decreases autocorrelation lengths, especially when the underlying distribution does not have complicated geometrical features or multimodalities. We use four times as many walkers as parameters. The cost of the affine-invariant method, which becomes more significant for larger parameter spaces, is that the time for the ensemble of walkers to equilibrate can be long. In our simulation, equilibration of an ensemble of walkers can require several days of computing time. However, once the ensemble is equilibrated, the autocorrelation length is small in comparison (half a day of computing time). One can create an equilibrated ensemble on only one thread, and then copy that equilibrated ensemble to many threads before simulating in parallel. We also spread out our walkers for one ensemble over many OpenMP threads, but to avoid complexities associated with multiple threads accessing or modifying the same walker at the same time, walkers are only updated after all walkers in the ensemble have undergone a "stretch move" (in the parlance of Ref. [30]). This slightly increases the autocorrelation length, but the OpenMP parallelization benefit far outweighs this cost. The MPI parallelization is trivial, except for coordination to ensure that many MPI ranks do not read or write from disk at the same time.

The folding of the data with the Gaussian in Eq. (1) can be handled with the use of FFTs. However, doing this directly for each neutron star at each Monte Carlo point is time-consuming. Thus, we cache the result of the FFT over a wide range of values for the intrinsic scattering parameter, generating a data cube covering $R$, $M$ and $\sigma$ for each source. We use linear interpolation in this data cube at each point to compute the conditional probability described above. The 8 simulations required about 500k core-hours of computational time.

# FURTHER RESULTS

Table II contains a tabulated version of Fig. 1 in the main paper.

## Tidal deformabilities in GW170817

The posteriors for the tidal deformabilities for the two stars in the GW170817 merger are given in Fig. 1. Panels (g) and (h) are slightly different, corresponding to slightly different EOS information, and this is comparable with the variation shown in Fig. 10 in Ref. [7]. Adding the X-ray data shrinks the posteriors significantly, and now the posteriors for the tidal deformabilities are less sensitive

| Model & data | $-2\sigma$ | $-1\sigma$ | med. | $+1\sigma$ | $+2\sigma$ |
|---|---|---|---|---|---|
| (a) 3P, GW | 11.30 | 11.59 | 12.17 | 13.33 | 13.95 |
| (b) 4L, GW | 10.65 | 11.25 | 11.77 | 12.36 | 13.09 |
| (c) 3P, GW, QLMXB, PRE | 11.21 | 11.69 | 11.93 | 12.29 | 12.55 |
| (d) 4L, GW, QLMXB, PRE | 11.27 | 11.65 | 11.88 | 12.10 | 12.31 |
| (e) 3P, all | 11.28 | 11.72 | 12.03 | 12.30 | 12.58 |
| (f) 4L, all | 11.32 | 11.67 | 11.93 | 12.12 | 12.34 |
| (g) 3P, all+IS | 11.18 | 11.6 | 11.98 | 12.39 | 12.75 |
| (h) 4L, all+IS | 11.12 | 11.54 | 11.83 | 12.14 | 12.45 |

TABLE II. The median ("med.") and $1\sigma$ and $2\sigma$ credible intervals for the radius of a 1.4 $M_\odot$ NS in km. Rows 7 and 8 include all the electromagnetic (EM) constraints (QLMXB, PRE, & NICER), convolved with intrinsic scattering (IS).

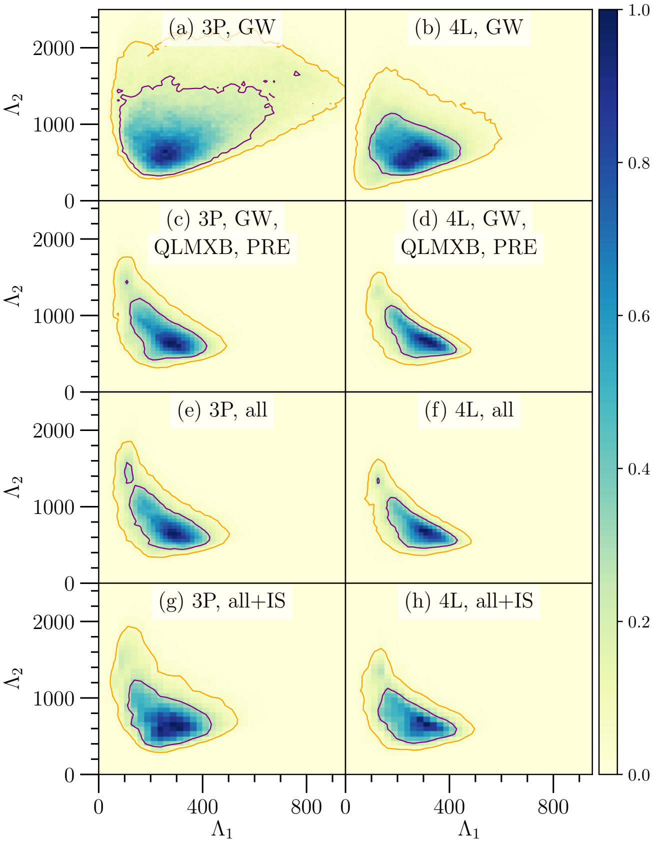


FIG. 1. Joint posterior distribution for $\Lambda_2$ and $\Lambda_1$ density plot with contour lines which enclose 68% or 95% of the probability distribution. Left panels are constructed with the "3P" EOS and right panels with the "4L" EOS. Different rows refer to different data selections. In each panel, the density plot is renormalized so that the peak is at 1.

to the addition of the data set or the EOS choice, as seen in panels (a), (b), (c) and (d).

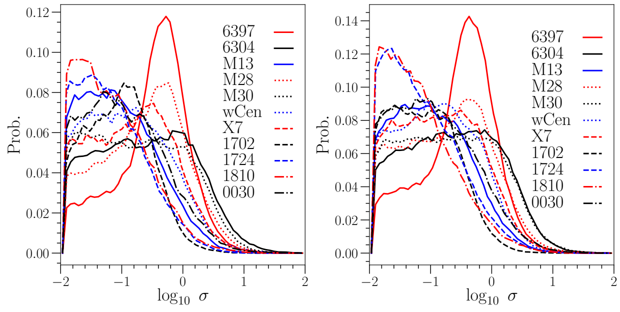


FIG. 2. The normalized posterior distributions for the intrinsic scattering parameters.

### Intrinsic Scattering Parameters

The posterior distributions for the intrinsic scattering parameters provide insight into which objects are most likely to contain systematic uncertainties (Fig. 2). The small radius implied when an H atmosphere is fit to the neutron star in NGC 6397 gives it a larger probability of a larger value of $\sigma$. Previous work on QLMXBs [1] also found that this object was more difficult to fit. The QLMXB and NICER objects generally have larger intrinsic scattering parameters than the PRE objects, but this may originate from the small size of our data set.

### Tidal Deformability Correlations

There are correlations and/or universal relations which have been used to analyze observations which constrain neutron star structure. We can test the validity of these assumptions in the context of our EOS parameterizations.

Ref. [31] showed that there is a correlation between the symmetric tidal parameter ($\Lambda_\mathrm{s} = \Lambda_2 + \Lambda_1$) and the antisymmetric part ($\Lambda_\mathrm{a} = \Lambda_2 - \Lambda_1$)

$$\Lambda_\mathrm{a,YY} = F_\mathrm{n}^{(\Lambda_\mathrm{a})}(q)\Lambda_\mathrm{s}^{-\alpha}\frac{a + \sum_{\mathrm{i}=1}^{3}\sum_{\mathrm{j}=1}^{2} b_\mathrm{ij} q^\mathrm{j} \Lambda_\mathrm{s}^{-\mathrm{i}/5}}{a + \sum_{\mathrm{i}=1}^{3}\sum_{\mathrm{j}=1}^{2} c_\mathrm{ij} q^\mathrm{j} \Lambda_\mathrm{s}^{-\mathrm{i}/5}} \qquad (9)$$

where

$$F_\mathrm{n}^{(\Lambda_\mathrm{a})}(q) \equiv \frac{1 - q^{10/(3-\mathrm{n})}}{1 + q^{10/(3-\mathrm{n})}}\,, \qquad (10)$$

and the values of the parameters $a$, $\alpha$, $b_{ij}$, $c_{ij}$, and $n$, are given in Ref. [31]. We compare $\Lambda_\mathrm{a,YY}$ with the exact value $\Lambda_\mathrm{a}$ in Fig. 3. We find that $\Lambda_\mathrm{a,YY}$ is generally an overestimate, with deviations as large as 30%. This effect may come from the fact that they use an EOS library that has many EOSs with smaller radii, and our observational constraints restrict us from sampling this part of the parameter space. Presuming this correlation is exact will tend to underestimate $\Lambda_a$. These deviations

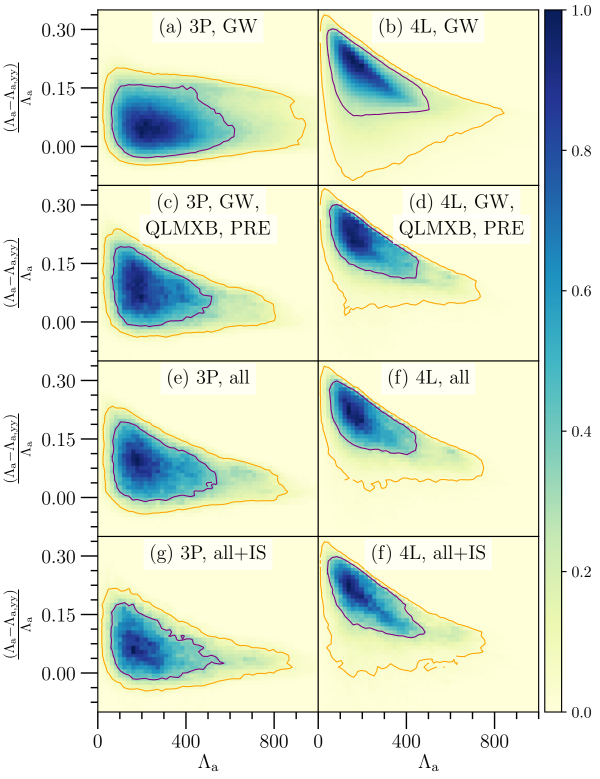


FIG. 3. Joint posterior distribution for the relative deviation between $\Lambda_{\rm a,YY}$ and $\Lambda_{\rm a}$ versus $\Lambda_{\rm a}$ with contour lines which enclose 68% or 95% of the probability distribution. Panel labeling follows Fig. 1.

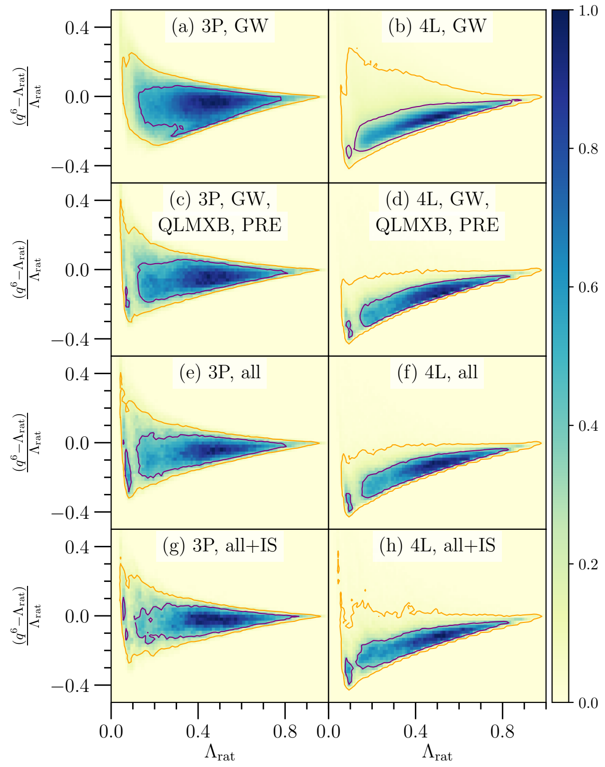


FIG. 4. Joint posterior distribution for the relative deviation between $q^6$ and $\Lambda_{\rm rat}$ versus $\Lambda_{\rm a}$ with contour lines which enclose 68% or 95% of the probability distribution. Panel labeling follows Fig. 1.

are different in the two EOS models, and in the 4L model they tend to be larger for smaller values of $\Lambda_a$.

Ref. [32] found that the ratio of the dimensionless tidal deformabilities, $\Lambda_{\rm rat} \equiv \Lambda_1/\Lambda_2$, is approximately equal to $q^6$ and we test this assumption in Fig. 4. Similar to the results for $\Lambda_{\rm a,YY}$, we find deviations as large as 40% and deviations that differ between the two EOS models. In effect, these assumptions are not independent of the EOS prior distribution. Presuming $\Lambda_{\rm rat} = q^6$ will tend to overestimate $\Lambda_{\rm rat}$.

Ref. [33] found a correlation between the compactness and tidal deformability of NS

$$\begin{aligned} C_{\rm i} =& 3.71 \times 10^{-1} - 3.91 \times 10^{-2} \ln \Lambda_{\rm i} \\ &+ 1.056 \times 10^{-3} (\ln \Lambda_{\rm i})^2 \end{aligned} \tag{11}$$

where i $= \{1, 2\}$ represents the NS in the binary. In Figs. 5 and 6 we compared the compactness ($C_{\rm exact}$) of the binaries from our posteriors with the relation provided in Eq. (11). We find that this correlation holds for the more massive neutron star to within about 3%, with a peak deviation which depends on the EOS model. For the less massive star, Eq. (11) can be an 8% overestimate; see also an updated analysis on the relationship between $C$ and $\Lambda$ in Ref. [29].

**Radius Correlations**

There is a well-known correlation between the symmetry energy slope parameter $L$ and the radius of a 1.4 solar mass neutron star [34], and it has been pointed out previously [28] that this correlation is dependent on the EOS prior distribution. Our joint posteriors are plotted in Fig. 7. The addition of the EM data weakens the correlation, in part simply because of the strong constraint

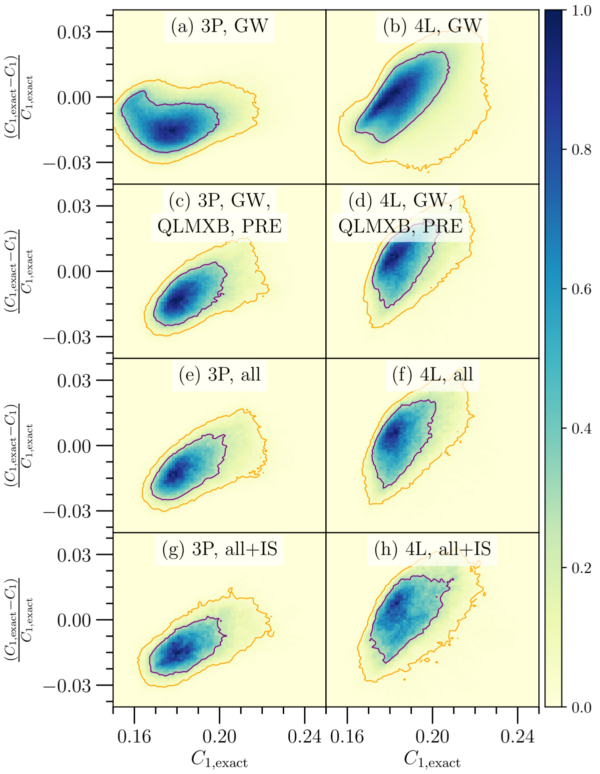


FIG. 5. Joint posterior distribution for the relative deviation between $C_1$ and $C_{\mathrm{exact},1}$ versus $C_{\mathrm{exact},1}$ with contour lines which enclose 68% or 95% of the probability distribution. Panel labeling follows Fig. 1.

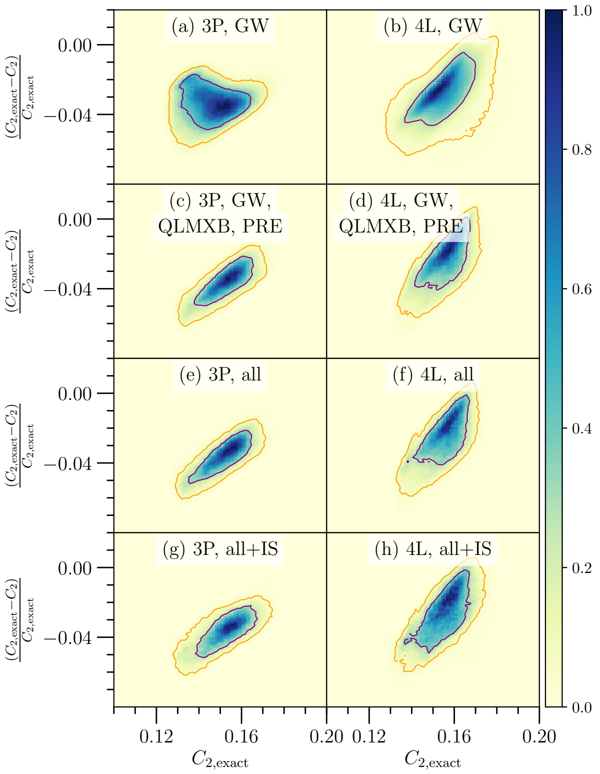


FIG. 6. Joint posterior distribution for the relative deviation between $C_2$ and $C_{\mathrm{exact},2}$ versus $C_{\mathrm{exact},2}$ with contour lines which enclose 68% or 95% of the probability distribution. Panel labeling follows Fig. 1.

| Model | $M_{\mathrm{max}}$ vs $R_{1.4}$ | $L$ vs $R_{1.4}$ |
|---|---|---|
| (a) 3P, GW | 0.397 | 0.842 |
| (b) 4L, GW | 0.420 | 0.704 |
| (c) 3P, GW, QLMXB, PRE | 0.315 | 0.558 |
| (d) 4L, GW, QLMXB, PRE | 0.167 | 0.436 |
| (e) 3P, all | 0.283 | 0.575 |
| (f) 4L, all | 0.109 | 0.454 |
| (g) 3P, all+IS | 0.381 | 0.667 |
| (h) 4L, all+IS | 0.175 | 0.496 |

TABLE III. Pearson correlation coefficients comparing the radius of a 1.4 solar mass neutron star with the slope of the symmetry energy, $L$, and the neutron star maximum mass.

on $R$. A similar correlation has also been suggested between maximum mass of neutron star $M_{\mathrm{max}}$ and the corresponding radius [35], but we find this correlation is relatively weak. Pearson correlation coefficients for these two correlations is $M_{\mathrm{max}}$ are given in Table III. The correlations are weaker in the 4L parameterization and the slope of the correlation also depends on the EOS parameterization.

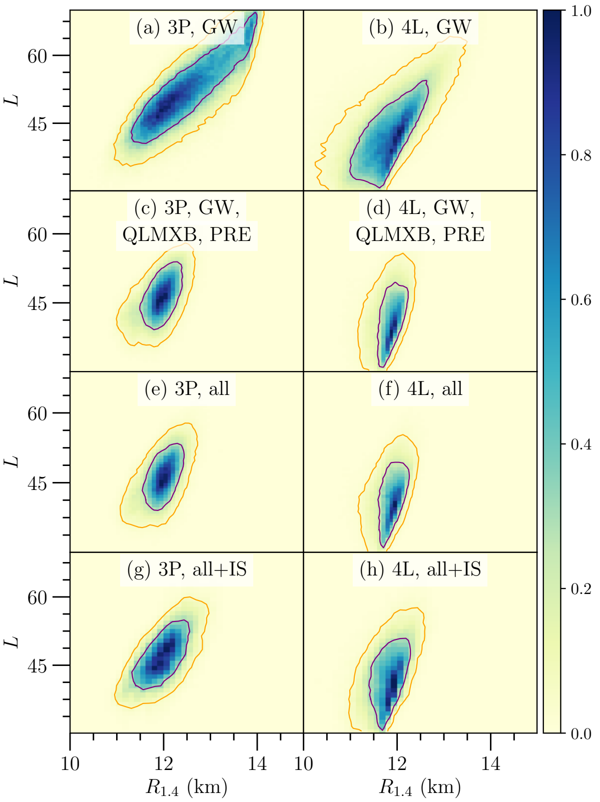


FIG. 7. Distributions for the cross correlation of EOS parameter $L$ with $R_{1.4}$. 3P models have weak correlations of these parameters. But, radius measured in 4L models are nearly independent of EOS parameters.

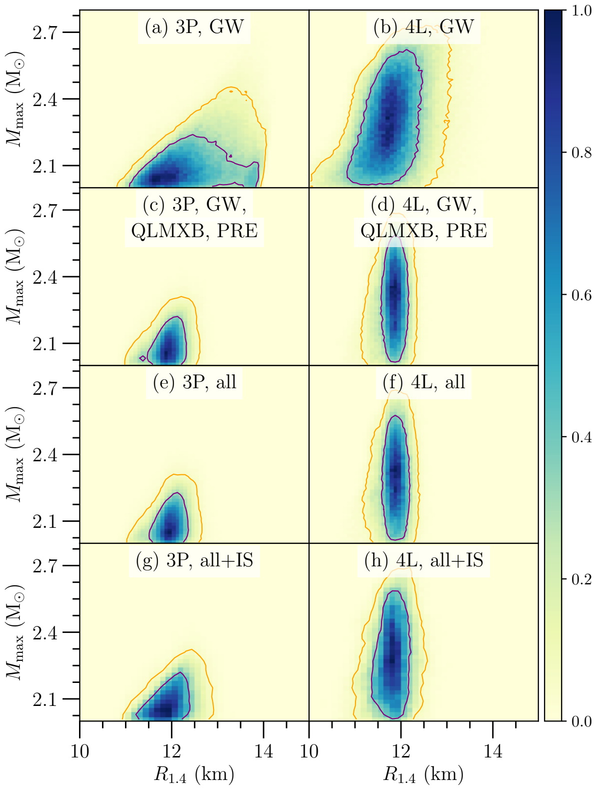


FIG. 8. Plots showing the cross correlation of $M_{\max}$ with $R_{1.4}$. 3P and 4L models with the combined analysis of GW and EM data are independent of these parameters.

[1] A. W. Steiner, C. O. Heinke, S. Bogdanov, C. Li, W. C. G. Ho, A. Bahramian, and S. Han, Mon. Not. Roy. Astron. Soc. **476**, 421 (2018), URL https://doi.org/10.1093/mnras/sty215.

[2] A. W. Shaw, C. O. Heinke, A. W. Steiner, S. Campana, H. N. Cohn, W. C. G. Ho, P. M. Lugger, and M. Servillat, Mon. Not. Roy. Astron. Soc. **476**, 4713 (2018), URL https://doi.org/10.1093/mnras/sty582.

[3] J. Nättilä, A. W. Steiner, J. J. E. Kajava, V. F. Suleimanov, and J. Poutanen, Astron. Astrophys. **591**, A25 (2016), URL https://doi.org/10.1051/0004-6361/201527416.

[4] J. Nättilä, M. C. Miller, A. W. Steiner, J. J. E. Kajava, V. F. Suleimanov, and J. Poutanen, Astron. and Astrophys. **608**, A31 (2017), URL https://doi.org/10.1051/0004-6361/201731082.

[5] T. E. Riley, A. L. Watts, S. Bogdanov, P. S. Ray, R. M. Ludlam, S. Guillot, Z. Arzoumanian, C. L. Baker, A. V. Bilous, D. Chakrabarty, et al., Astrophys. J. **887**, L21 (2019), URL https://doi.org/10.3847/2041-8213/ab481c.

[6] M. C. Miller et al., Astrophys. J. **887**, L24 (2019), URL https://doi.org/10.3847/2041-8213/ab50c5.

[7] LIGO Scientific Collab. and Virgo Collab., Phys. Rev. Lett. **121**, 161101 (2018), URL https://doi.org/10.1103/PhysRevLett.121.161101.

[8] J. Lange, R. O'Shaughnessy, and M. Rizzo, arXiv:1805.10457 (2018), URL https://arxiv.org/abs/1805.10457.

[9] A. W. Steiner, arXiv:1802.05339 (2018), URL https://arxiv.org/abs/1802.05339.

[10] S. Gandolfi, J. Lippuner, A. W. Steiner, I. Tews, X. Du, and M. Al-Mamun, J. Phys. G. (2019), URL https://doi.org/10.1088/1361-6471/ab29b3.

[11] X. Du, A. W. Steiner, and J. W. Holt, Phys. Rev. C **99**, 025803 (2019), URL https://doi.org/10.1103/PhysRevC.99.025803.

[12] S. Gandolfi, J. Carlson, and S. Reddy, Phys. Rev. C **85**, 032801 (2012), URL https://doi.org/10.1103/PhysRevC.85.032801.

[13] J. Lynn, I. Tews, J. Carlson, S. Gandolfi, A. Gezerlis, K. Schmidt, and A. Schwenk, Phys. Rev. Lett. **116**, 062501 (2016), URL https://doi.org/10.1103/PhysRevLett.116.062501.

[14] A. Gezerlis, I. Tews, E. Epelbaum, M. Freunek, S. Gandolfi, K. Hebeler, A. Nogga, and A. Schwenk, Phys. Rev. C **90**, 054323 (2014), URL https://doi.org/10.1103/PhysRevC.90.054323.

[15] I. Tews, S. Gandolfi, A. Gezerlis, and A. Schwenk, Phys. Rev. C **93**, 024305 (2016), URL https://doi.org/10.1103/PhysRevC.93.024305.

[16] K. E. Schmidt and S. Fantoni, Phys. Lett. B **446**, 99 (1999), URL https://doi.org/10.1016/S0370-2693(98)01522-6.

[17] J. D. McDonnell, N. Schunck, D. Higdon, J. Sarich, S. M. Wild, and W. Nazarewicz, Phys. Rev. Lett. **114**, 122501 (2015), URL https://doi.org/10.1103/PhysRevLett.114.122501.

[18] M. Kortelainen, J. McDonnell, W. Nazarewicz, E. Olsen, P.-G. Reinhard, J. Sarich, N. Schunck, S. M. Wild, D. Davesne, J. Erler, et al., Phys. Rev. C **89**, 054314 (2014), URL https://doi.org/10.1103/PhysRevC.89.054314.

[19] A. W. Steiner, J. M. Lattimer, and E. F. Brown, Astrophys. J. **722**, 33 (2010), URL https://doi.org/10.1088/0004-637X/722/1/33.

[20] M. F. Carney, L. E. Wade, and B. S. Irwin, Phys. Rev. D **98**, 063004 (2018), URL https://doi.org/10.1103/PhysRevD.98.063004.

[21] R. C. Tolman, Phys. Rev. **55**, 364 (1939), URL https://doi.org/10.1103/PhysRev.55.364.

[22] J. Oppenheimer and G. Volkoff, Phys. Rev. **55**, 374 (1939), URL https://doi.org/10.1103/PhysRev.55.374.

[23] P. B. Demorest, T. Pennucci, S. M. Ransom, M. S. E. Roberts, and J. W. T. Hessels, Nature (London) **467**, 1081 (2010), URL https://dx.doi.org/10.1038/nature09466.

[24] J. Antoniadis, P. C. C. Freire, N. Wex, T. M. Tauris, R. S. Lynch, M. H. van Kerkwijk, M. Kramer, C. Bassa, V. S. Dhillon, T. Driebe, et al., Science **340**, 6131 (2013), URL https://doi.org/10.1126/science.1233232.

[25] H. T. Cromartie, E. Fonseca, S. M. Ransom, P. B. Demorest, Z. Arzoumanian, H. Blumer, P. R. Brook, M. E. DeCesar, T. Dolch, J. A. Ellis, et al., Nature Astron. **4**, 72 (2020), URL https://doi.org/10.1038/s41550-019-0880-2.

[26] J. B. Hartle, Astrophys. Supp. Ser. **24**, 385 (1973), URL https://doi.org/10.1007/BF02637163.

[27] K. Yagi and N. Yunes, Science **341**, 365 (2013), URL https://doi.org/10.1126/science.1236462.

[28] A. W. Steiner, J. M. Lattimer, and E. F. Brown, Eur. Phys. J. A **52**, 18 (2016), URL https://doi.org/10.1140/epja/i2016-16018-1.

[29] Z. Carson, K. Chatziioannou, C.-J. Haster, K. Yagi, and N. Yunes, Phys. Rev. D **99**, 083016 (2019), URL https://doi.org/10.1103/PhysRevD.99.083016.

[30] J. Goodman and J. Weare, Comm. App. Math. and Comp. Sci. **5**, 65 (2010), URL https://doi.org/10.2140/camcos.2010.5.65.

[31] K. Yagi and N. Yunes, Classical and Quantum Gravity **34**, 015006 (2016), URL https://doi.org/10.1088/1361-6382/34/1/015006.

[32] S. De, D. Finstad, J. M. Lattimer, D. A. Brown, E. Berger, and C. M. Biwer, Phys. Rev. Lett. **121**, 091102 (2018), URL https://doi.org/10.1103/PhysRevLett.121.091102.

[33] A. Maselli, V. Cardoso, V. Ferrari, L. Gualtieri, and P. Pani, Phys. Rev. D **88**, 023007 (2013), URL https://doi.org/10.1103/PhysRevD.88.023007.

[34] J. M. Lattimer and M. Prakash, Astrophys. J. **550**, 426 (2001), URL https://doi.org/10.1086/319702.

[35] C. D. Capano, I. Tews, S. M. Brown, B. Margalit, S. De, S. Kumar, D. A. Brown, B. Krishnan, and S. Reddy, Nature News (2020), URL https://doi.org/10.1038/s41550-020-1014-6.
